# Supplementary material for: Handling Long-Term Safety and Uncertainty in Safe Reinforcement Learning
Source: arXiv:2409.12045 source file (2024-09-23)
Supplement: Supplementary file 1 [file 0_deprecated.tex]

\section{Extensions}
\subsection{k-step feasibility}
We can extend the concept of \gls{fvf} the setting of limited return. We define a \gls{kfvf} as 
\begin{equation*}
    \FeasibilityValue^{\Policy, k}(\State) = \expect{\Policy}{\left.\sum_{t=0}^{k} \gamma^t \max(\Constr(\State_t), 0) \right| \State_0 = \State} \label{eq:feasibility_value_k}
\end{equation*}
Similarly to the \gls{fvf}, also the \gls{kfvf}   $\FeasibilityValue^{\Policy, k}\in [0, \frac{1 - \Discount ^K }{1 - \Discount}\Constr_{\max}]$ is bounded if the constraint $\Constr(\State)\in[\Constr_{\min} , \Constr_{\max} ]$ is bounded. 

\subsection{Learning simple constraints}
In some settings, learning a Feasibility Value Function is not necessary, as the local constraint satisfaction is sufficient to ensure safety. This setting is common when the controlled robot can be described as a first-order system.
In this setting, we can train $\Constr_{\theta}(\State)$ and $V_{F, \phi}^{\Policy}(\State)$ simultaneously using the following loss
\begin{equation*}
    \Loss_{\Constr} = \Vert \Constr(\State) - \Constr_{\theta}(\State) \Vert^2 
\end{equation*}
where $\Loss_{\Constr}$ minimizes the mean squared error of the constraint approximation. 

Also in this setting, we can consider the stochastic formulation of the constraint. To obtain the stochastic version, we train the constraint function $\Constr_{\theta}(\State)$ using the negative log-likelihood loss
\begin{equation}
    \Loss_{\theta} = -\log \Normal(\Constr(\State); \mu_\theta^{\Constr}(\State), \Sigma_\theta^{\Constr}(\State)) 
    \label{eq:loss_constraint}
\end{equation}

We model the distribution of the constraint $\widehat{\Constr}(\State)$ as a Gaussian distribution with mean $\mu^{\widehat{\Constr}}(\State)$ and variance $\Sigma^{\widehat{\Constr}}(\State)$. The $\var_\alpha^{\widehat{h}}(\State)$ and $\cvar_\alpha^{\widehat{h}}(\State)$ has a closed-form solution as
\begin{align}
    \var_\alpha^{\widehat{h}}(\State) &= \mu^{\widehat{\Constr}}(\State) + \Phi^{-1}(\alpha) \sqrt{\Sigma^{\widehat{\Constr}}(\State)} \nonumber\\
    \cvar_\alpha^{\widehat{h}}(\State) &= \mu^{\widehat{\Constr}}(\State) + \frac{\psi(\Psi^{-1}(\alpha))}{1 - \alpha} \sqrt{\Sigma^{\widehat{\Constr}}(\State)} \label{eq:cvar_constraint}
\end{align}
where $\Psi(\cdot)$ and $\psi(\cdot)$ are the \gls{cdf} and \gls{pdf} of the standard normal distribution. $\Phi^{-1}(\cdot)$ is the inverse function of \gls{cdf}.
%Training $\Constr_{\theta}(\State)$ and $V_{F, \phi}^{\Policy}(\State)$ separately is beneficial as $\Constr_{\theta}(\State)$ trained with supervised learning has a faster convergence rate and lower approximation error. Leveraging the information of $\Constr_\theta(\State)$ to obtain a safe policy will result in fewer constraint violations during training.
